# Supplementary material for: Searching for Decoherence from Quantum Gravity at the IceCube South Pole Neutrino Observatory
Source: arXiv:2308.00105 source file (2023-07-25)
Supplement: Supplementary file 1 [file Appendix.tex]

\documentclass[pdflatex,sn-mathphys,iicol,lineno]{sn-jnl}% 

\jyear{2023}%
\theoremstyle{thmstyleone}%
\newtheorem{theorem}{Theorem}% meant for continuous numbers
\newtheorem{proposition}[theorem]{Proposition}% 
\theoremstyle{thmstyletwo}%
\newtheorem{example}{Example}%
\newtheorem{remark}{Remark}%
\theoremstyle{thmstylethree}%
\newtheorem{definition}{Definition}%
\raggedbottom
%%\unnumbered% uncomment this for unnumbered level heads
\usepackage{physics}
\newcommand\headercell[1]{%
   \smash[b]{\begin{tabular}[t]{@{}c@{}} #1 \end{tabular}}}
\usepackage{adjustbox}
\usepackage[font=scriptsize]{caption}

\begin{document}
